# Supplementary material for: Optimizing Drivers' Discount Order Acceptance Strategies: A Policy-Improved Deep Deterministic Policy Gradient Framework
Source: arXiv:2507.11865 source file (2025-12-11)
Supplement: Supplementary file 1 [file appendix.tex]

\section*{Appendix A. Nomenclature}

\setcounter{table}{0}

\begin{table}[!ht]
	\footnotesize
	\centering
	\caption{Notations for I-OFOMAC}
	\begin{tabularx}{\textwidth}{lX}
		\toprule
		\textbf{Notations} & \textbf{Explanation} \\
		\midrule
		\multicolumn{2}{l}{\textit{Sets}} \\
		$\mathcal G$ & The directed graph of road network\\
		$\mathcal N$ & The set of network nodes\\
		$\mathcal L$ & The set of network links\\
		$\mathcal L_E$ & The set of links with temporal waiting zones alongside \\
		$\mathcal K_\tau$ & The set of vacant SAVs in cycle $\tau$: $k\in \mathcal K$ \\
		$\mathcal P_\tau$ & The set of customers in cycle $\tau$: $p\in \mathcal P$ \\
            $\mathcal P'_\tau$ & The set of customers who are expected to leave the system without getting response after cycle $\tau$\\
		$\mathcal V_\tau$ & The set of PAVs in cycle $\tau$: $v\in \mathcal V$ \\
		$\mathcal U$ & The set of virtual platoons: $u_{i,j,t} \in \mathcal U$, where $u_{i,j,t}$ denotes the virtual platoon connecting nodes $i$ and $j$ in cycle $t$ \\
		$\hat{R}^{W_v}$ & The set of candidate routes for PAV $v$ \\
		$\hat{R}^{W_k}_p$ & The set of candidate  routes for SAV $k$ to serve customer  $p$ \\
		$\mathcal S$ & The state space for the MDP: $s = (t,l) \in \mathcal S$ \\	
		$\mathcal B$ & The historical transition set: $(s_i, a_i, R_{\gamma, i}, s_i')\in \mathcal B$ \\
		& \\
		\multicolumn{2}{l}{\textit{Parameters}} \\
		$\tilde{T}$ & The cycle length of space-time network \\
		$\alpha$ & The parameter indicating the priority of the SAV platform in the integrated operations \\
		$\beta$ & The stability parameter in the modified state value network with extra bonus \\
		$\gamma$ & The discount factor for the MDP \\
		$\epsilon$ & The exploration rate for the DRL \\
		$\theta$ & The parameter of the neural network approximating the state value \\
		$\mu$ & The parameter indicating the value of travel time \\
		$\phi$ & The parameter of the neural network approximating the bisimulation metric \\
		& \\
		\multicolumn{2}{l}{\textit{Variables}} \\
		$R_p$ & The service fee for customer $p$ \\
		$R_\gamma(p,r,q)$ & The discounted reward of serving customer $p$ with route $r$ and start cycle $q$ \\
		$V(s \mid \theta)$ & The state value for state $s$ parameterized by $\theta$ \\
		$b(s,s'\mid \phi)$ & The bisimulation metric between states $s$ and $s'$ parameterized by $\phi$ \\
		$Q_s(k,p,r,q)$ & The action value of SAV $k$ serving customer $p$ with route $r$ and start cycle $q$ \\
		$Q_i(k)$ & The action value of SAV $k$ remaining idle for one cycle \\
		$D$ & The maximum start cycle for each AV \\
		$C_p$ & The penalty to the SAV platform revenue for not responding to customer $p$ \\
		$c_{r,q}$ & The travel time of route $r$ with start cycle $q$ \\
		$E^{i,j,t}_\tau$ & The remaining capacity of virtual platoon $u_{i,j,t}$ at the beginning of cycle $\tau$\\
		$\sigma^{i,j,t}_{r,q}$ & The 1-0 variable indicating whether route $r$ with start cycle $q$ occupies one unit capacity of virtual platoon $u_{i,j,t}$ or not \\
		& \\
		\multicolumn{2}{l}{\textit{Decision variables}} \\
		$x_{k,p,r,q}$ & The 1-0 decision variable indicating whether SAV $k$ is matched with customer $p$ with service route $r$ and start cycle $q$ \\
		$x_{v,r,q}$ & The 1-0 decision variable indicating whether PAV $v$ travels along route $r$ with start cycle $q$ \\
		$y_{p}$ & The 1-0 decision variable indicating whether respond to customer $p$ or not \\
		$z_k$ & The 1-0 decision variable indicating whether SAV $k$ remains idle for one cycle \\
		\bottomrule
	\end{tabularx}
	\label{Notataion_tab}
\end{table}
